# Supplementary material for: A Fast Heuristic for Computing Geodesic Cores in Large Networks
Source: arXiv:2206.07350 source file (2022-06-15)
Supplement: Supplementary file 1 [file appendix.tex]

%.\main.tex
% !TeX spellcheck = en_US
\clearpage
\appendix
\section{Supplementary Materials: Proofs}\label{sec:proofs}

%\begin{proof}[Proof of \Cref{lm:correctnessblockclosure}]
%	The correctness is immediate from Thm.~\ref{thm:outerplanar_preclosure}, Lemma~\ref{lm:generatorset}, and the correctness of computing all shortest paths between a vertex and a set of vertices of a graph by BFS.	
%	Regarding the complexity, by Lemma~\ref{lm:generatorset} we have that $G_X$ is of size $\bigO{f}$ and can be calculated in $\bigO{n}$ time.
%	Furthermore, each BFS call in line~\ref{alg:BFScall} can be performed in $\bigO{n}$ time, as $|E(B)| = \bigO{n}$.
%	Thus, the total time is bounded by $\bigO{nf}$ as claimed.
%\end{proof}	
